# Supplementary material for: Hyperfine-interaction limits polarization entanglement of photons from semiconductor quantum dots
Source: arXiv:2302.05983 source file (2023-04-27)
Supplement: Supplementary file 1 [file Supplementary.pdf]

# Hyperfine-interaction limits polarization entanglement of photons from semiconductor quantum dots

Christian Schimpf,<sup>1</sup> Francesco Basso Basset,<sup>2</sup> Maximilian Aigner,<sup>1</sup> Wolfgang  
Attenender,<sup>1</sup> Laia Gínes,<sup>3</sup> Gabriel Undeutsch,<sup>1</sup> Marcus Reindl,<sup>1</sup> Daniel  
Huber,<sup>1</sup> Dorian Gangloff,<sup>4</sup> Evgeny A. Chekhovich,<sup>5</sup> Christian Schneider,<sup>6</sup>  
Sven Höfling,<sup>7</sup> Ana Predojević,<sup>3</sup> Rinaldo Trotta,<sup>2</sup> and Armando Rastelli<sup>1</sup>

<sup>1</sup>*Institute of Semiconductor and Solid State Physics,  
Johannes Kepler University Linz, 4040 Linz, Austria \**

<sup>2</sup>*Department of Physics, Sapienza University of Rome, 00185 Rome, Italy*

<sup>3</sup>*Department of Physics, Stockholm University, 106 91 Stockholm, Sweden*

<sup>4</sup>*Department of Engineering Science,  
University of Oxford, Oxford, OX1 3PJ, United Kingdom*

<sup>5</sup>*Department of Physics and Astronomy,  
University of Sheffield, United Kingdom*

<sup>6</sup>*Institute of Physics, Carl von Ossietzky Universität Oldenburg, 26111 Oldenburg, Germany*

<sup>7</sup>*Technische Physik and Wilhelm Conrad Röntgen  
Research Center for Complex Material Systems,  
Universität Würzburg, 97074 Würzburg, Germany*

(Dated: February 17, 2023)

## I. THEORETICAL CONSIDERATIONS

## II. NUMERICAL MODEL

The Hamiltonian of a heavy-hole excitons (X) in a quantum dot (QD) in the basis of the total angular momentum projection in the  $z$ -direction (here: the growth direction)  $\{|+1\rangle, |-1\rangle, |+2\rangle, |-2\rangle\}$  is given by [1, 2]:

$$H_X = \begin{pmatrix} \delta_0 - h_{z-} & \delta_1 & h_e & h_h \\ \delta_1^* & \delta_0 + h_{z-} & h_h^* & h_e \\ h_e^* & h_h & -\delta_0 + h_{z+} & \delta_2 \\ h_h^* & h_e^* & \delta_2^* & -\delta_0 - h_{z+} \end{pmatrix} \quad (1)$$

with  $\delta_0$  being equal to half of the bright-dark exciton splitting,  $\delta_{1,2} \in \mathbb{C}$  having an absolute value equal to half of the energy splittings between the bright (dark) excitons  $\{|+1\rangle, |-1\rangle\}$  ( $\{|+2\rangle, |-2\rangle\}$ ) and  $h_{e(h)} = h_{e(h)}^x + ih_{e(h)}^y$ , with  $h_{e(h)}^{x,y}$  the electron- (hole-) hyperfine shifts in the  $x$ - and  $y$ -directions and  $h_{z\pm} = h_e^z \pm h_h^z$  the hyperfine shift in the  $z$  direction.

In the QDs under investigation  $\delta_0$  typically lies in the range of 50  $\mu\text{eV}$ , which is much larger than  $S$  or the OS at play, so that we can separate out the bright X states via a Schrieffer-Wolf transformation [2]:

$$\tilde{H}_X = \tilde{H}_0 + \tilde{H}_2 \quad (2)$$

$$\tilde{H}_0 = \frac{1}{2} \begin{pmatrix} \delta_0 - h_{z-} & \delta_1 \\ \delta_1^* & \delta_0 + h_{z-} \end{pmatrix} \quad (3)$$

$$\tilde{H}_2 = \frac{1}{4} \begin{pmatrix} \frac{|h_e|^2}{\delta_0 - b_e} + \frac{|h_h|^2}{\delta_0 + b_h} & \frac{\delta_0 h_e h_h^*}{\delta_0^2 - b_e^2} + \frac{\delta_0 h_e h_h^*}{\delta_0^2 - b_h^2} \\ \frac{\delta_0 h_e^* h_h}{\delta_0^2 - b_e^2} + \frac{\delta_0 h_e^* h_h}{\delta_0^2 - b_h^2} & \frac{|h_e|^2}{\delta_0 + b_e} + \frac{|h_h|^2}{\delta_0 - b_h} \end{pmatrix}, \quad (4)$$

with  $b_{e(h)} = h_{e(h)}^z$ . For the assumed  $\delta_0$ ,  $\tilde{H}_2$  can safely be neglected, as was done for the calculations in the main paper. Further, we neglected the hole contributions, as they typically account for about a tenth of the electron contribution [3], so that  $h_{z\pm} = h_z^e =: h_z$ . The energy splitting between  $|+1\rangle$  and  $|-1\rangle$  is then given by  $\delta_1 = S/2$ , with  $S$  the bright exciton fine

---

\* christian.schimpf@jku.at

structure splitting [1]. For one specific hyperfine shift  $h_z$  the time-evolution of the 2-qubit density matrix of the two photons emitted in the radiative XX-X decay cascade is given by:

$$i \hbar \frac{d}{dt} \rho_{h_z}(t) = \left[ \mathbb{I}^{(2)} \otimes \tilde{H}_X, \rho_{h_z}(t) \right], \quad (5)$$

with  $\mathbb{I}^{(2)}$  the  $2 \times 2$  identity matrix and  $\rho_{h_z}(0) = |\psi^+\rangle \langle \psi^+|$ . By discretizing the decay time of the exciton in  $N$  equidistant values  $t_i$ , the discrete probability density function of the X decay is given by

$$P(t_i) = \frac{e^{-t_i/T_1}}{\sum_{k=0}^{N-1} e^{-t_k/T_1}}, \quad (6)$$

with the X lifetime  $T_1$ . The times  $t_i$  are probed by a numerical Von-Neumann solver (from the “Qutip” Python library) with a spacing of  $T/N$  (with  $T$  the maximum probed X decay time). The time-averaged density matrix is then given by

$$\langle \rho_{h_z} \rangle_t = \sum_{i=0}^{N-1} P(t_i) \rho_{h_z(t_i)}. \quad (7)$$

$h_z$  is varied  $K$  times, each time with a random direction in  $\mathbb{R}^3$  and an amplitude sampled from a Gaussian distribution with a standard deviation of  $\sigma$ , which results in

$$\langle \rho \rangle_t = \frac{1}{K} \sum_{j=0}^{K-1} \bar{\rho}_{h_{zj}}. \quad (8)$$

The values in the main text were calculated by setting the time-steps from 0 to  $T = 5$  ns,  $N = 5000$ , and  $K = 600$ , in order to probe sufficiently many time steps and random configurations of  $h_z$ . For calculating the  $C$  values for Fig. 4(b),  $T$  was set to the used correlation window stated in the figure and  $N = 2000$ ;

### III. ANALYTICAL MODEL FOR THE TWO-PHOTON DENSITY MATRIX

In the basis given by  $X_{H/V} = \{(|+1\rangle \pm |-1\rangle)/\sqrt{2}\}$ , where  $|\pm 1\rangle$  are the eigenstates of the total electron-hole angular momentum along the  $z$ -direction, the Hamiltonian is given by [1]:

$$H = \begin{pmatrix} \delta_1 & \delta_2 \\ \delta_2^* & -\delta_1 \end{pmatrix} \quad (9)$$

where  $\delta_1 = S/2$  and  $\delta_2 = ih_z$ . The orthonormal eigenvectors of Eq. (9) in the photon polarization basis  $|H\rangle, |V\rangle$  are given as

$$(|j\rangle, |l\rangle) = \frac{1}{\nu} \begin{pmatrix} \sqrt{\frac{1}{2} + \frac{2\delta_1}{\Delta_E}} \nu & h_z^2 \\ ih_z & -i(\Delta_E + 2\delta_1) \end{pmatrix}, \quad (10)$$

with  $\nu = \sqrt{\Delta_E \delta_1 + 2h_z^2 + 2\delta_1^2}$ . The entangled XX-X state is given by

$$|\psi_{h_z}\rangle(t) = \frac{1}{\sqrt{2}} \left( |j^*\rangle \otimes |j\rangle + e^{-\frac{i}{\hbar} \Delta_E t} |l^*\rangle \otimes |l\rangle \right). \quad (11)$$

The complex conjugate (\*) mirrors the circular contribution of  $|j\rangle$  and  $|l\rangle$  (in the rectilinear basis!), corresponding to the angular momentum. As a consequence, regardless of  $|j\rangle$  and  $|l\rangle$ , the total angular momentum for each possible XX-X decay-path is conserved and the initial state results to  $|\psi_{h_z}\rangle(0) = |\phi^+\rangle$ . Proof:

$$\begin{aligned} |j\rangle &:= \begin{pmatrix} j_1 \\ j_2 \end{pmatrix}, |l\rangle := \begin{pmatrix} l_1 \\ l_2 \end{pmatrix}, \\ \langle j|j\rangle &= \langle k|k\rangle = 1, \\ \langle j|k\rangle &= j_1^* k_1 + j_2^* k_2 = 0, \\ \Rightarrow k &= \begin{pmatrix} j_2^* \\ -j_1^* \end{pmatrix}, \Rightarrow \frac{1}{2} (|j^*\rangle \otimes |j\rangle + |k^*\rangle \otimes |k\rangle) = \begin{pmatrix} 1 \\ 0 \\ 0 \\ 1 \end{pmatrix} \end{aligned} \quad (12)$$

Solving the eigenvalue problem for the Hamiltonian given by Eq. (9) results in the two orthonormal eigenstates  $|j\rangle, |l\rangle$ , with an energy difference of  $\Delta_E = 2\sqrt{\delta_1^2 + \delta_2^2}$ .

For a measurement duration much larger than  $\tau_S$ , and in the absence of time-filtering, we integrate the time-dependent state  $|\psi_{h_z}\rangle \langle\psi_{h_z}|(t)$  over the exponentially decaying emission probability of the exciton with a statistical lifetime of  $T_1$ . We set  $\hbar := 1$  to facilitate the

calculations.

$$\begin{aligned}
\langle \rho_{h_z} \rangle_t &= \int_0^\infty \frac{e^{-t/T_1}}{T_1} |\psi_{h_z}\rangle \langle \psi_{h_z}|(t) dt = \\
&= N_{h_z} \begin{pmatrix} 1 + 2T_1^2(h_z^2 + 2\delta_1^2) & -h_z T_1(2iT_1\delta_1 + 1) & h_z T_1(2iT_1\delta_1 + 1) & 1 + 2iT_1\delta_1 + 2h_z^2 T_1^2 \\ h_z T_1(2i\delta_1 T_1 - 1) & 2h_z^2 T_1^2 & -2h_z^2 T_1^2 & -h_z T_1(2i\delta_1 T_1 + 1) \\ -h_z T_1(2i\delta_1 T_1 - 1) & -2h_z^2 T_1^2 & 2h_z^2 T_1^2 & h_z T_1(2i\delta_1 T_1 + 1) \\ 1 - 2iT_1\delta_1 + 2h_z^2 T_1^2 & h_z T_1(2iT_1\delta_1 - 1) & -h_z T_1(2iT_1\delta_1 - 1) & 1 + 2T_1^2(h_z^2 + 2\delta_1^2) \end{pmatrix} \\
N_{h_z} &= \frac{1}{2 + 8T_1^2(\delta_1^2 + h_z^2)}
\end{aligned} \tag{13}$$

Further, we sample the amplitude of the OS from a normal distribution with a variance of  $\sigma^2$  and a mean value of zero:

$$\begin{aligned}
\langle \rho \rangle_t &= \int_{-\infty}^\infty \int_0^\infty \frac{\text{Exp}\left(-\frac{t}{T_1} - \frac{h_z^2}{2\sigma^2}\right)}{\sqrt{2\pi} T_1 \sigma} |\psi_{h_z}\rangle \langle \psi_{h_z}|(t) dt dh_z \\
&= \frac{1}{1 + 4T_1^2(S^2 + \sigma^2)} \begin{pmatrix} \frac{1}{2} + T_1^2(2S^2 + \sigma^2) & 0 & 0 & \frac{1}{2} + iT_1 S + T_1^2 \sigma^2 \\ 0 & T_1^2 \sigma^2 & -T_1^2 \sigma^2 & 0 \\ 0 & -T_1^2 \sigma^2 & T_1^2 \sigma^2 & 0 \\ \frac{1}{2} - iT_1 S + T_1^2 \sigma^2 & 0 & 0 & \frac{1}{2} + T_1^2(2S^2 + \sigma^2) \end{pmatrix}.
\end{aligned} \tag{14}$$

By indicating with  $k$  the fraction of events with no more than one photon pair per excitation cycle, we account for the multi-photon emission probability  $1 - k$  as in [4]:

$$1 - k \approx \frac{g_{\text{XX}}^{(2)}(0) + g_{\text{X}}^{(2)}(0)}{2} \eta_{\text{P}}. \tag{15}$$

By measuring the quantities in the above equation for each QD, we add a mixing channel to  $\langle \rho \rangle_t$  so that

$$\tilde{\rho} = k \langle \rho \rangle_t + \frac{1 - k}{4} \mathbb{I}^{(4)}, \tag{16}$$

with  $\mathbb{I}^{(4)}$  the  $4 \times 4$  identity matrix. From Eq. (16) we can derive an estimation for the fidelity to the  $|\phi^+\rangle$  Bell state as

$$f = \langle \phi^+ | \tilde{\rho} | \phi^+ \rangle = \frac{1}{4} \left( 1 + k + \frac{2k}{1 + 4T_1^2(S^2 + \sigma^2)/\hbar^2} \right). \tag{17}$$

In order to confirm the validity of the approximations for  $F$  made from Eq. (17), we compare the predicted values for  $f$  as a function of  $S$  against the ones calculated from Eq.

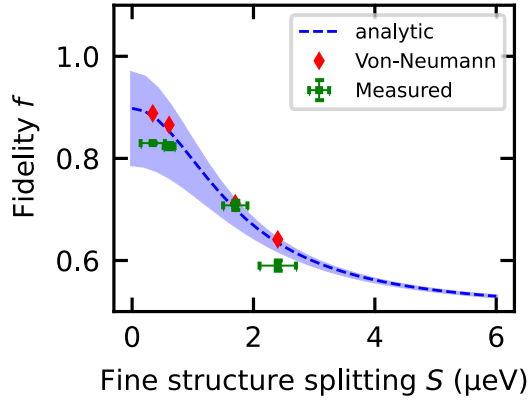

FIG. 1. Measured fidelity values of QD1p, for which the FSS was tuned to different values by the piezo-actuator (see main text). The blue line shows calculated fidelity for  $\sigma = 0.39 \mu\text{eV}$  ( $T_2^* = 1.7 \text{ ns}$ ) according to Eq. (17), the green squares depict the measured values. The red show the values calculated from Eq. (8) by drawing from 600 random OS configurations for each value of  $S$ .

(8), see Fig. 1. We observe that the values are in good agreement, and that Eq. (16) can safely be used to estimate  $f$ . However, in order to obtain a more accurate estimation of the 2-qubit density matrix, Eq. (8) should be preferred as it does not restrict the OS into the xz plane and therefore leads to a different distribution of the density matrix elements.

## IV. EXPERIMENTAL DETAILS

### A. Methods

The InGaAs quantum dots (QDs) used in this work were produced with the partial-capping-and-annealing method [5] and originate from the same wafer that was used for the pioneering work in Ref. [6]. The QD-containing GaAs layer is embedded in a distributed Bragg resonator consisting of 24 (bottom) and 5 (top) pairs of alternating  $\text{Al}_{0.9}\text{Ga}_{0.1}\text{As}$  and GaAs layers.

All the measurements are performed at a nominal temperature of 4 K in a helium-flow cryostat. The excitation is done with a mode-locked titanium-sapphire laser featuring a pulse duration of 100 fs and a repetition rate of 80 MHz passing a 4f pulse-shaper setup to

form ps-pulses (10 ps duration). The laser is focused via an objective (NA = 0.42) onto the sample. We use tunable notch filters in transmission with a bandwidth of 0.4 nm to reject scattered laser light. The transmission- and reflection outputs of the beam splitter (BS) were individually checked for polarization altering effects by performing Stokes vector measurements, resulting in negligible relative phase delays between the horizontal and the vertical optical axis. After fiber coupling of the QD signal, the light is guided to and spectrally filtered by spectrometers, where the signal is then either detected by a CCD camera or - during photon correlation spectroscopy - by avalanche photodiodes connected to the correlation electronics. The temporal resolution of these detectors used for the second-order correlations is about 350ps (40 dark counts per second). The lifetime measurements are performed by the use of another avalanche photodiode featuring 50ps temporal resolution. The measurements of the FSS are carried out with a rotating  $\lambda/2$  wave plate in front of a fixed polarizer placed at the entrance of a 1800 lines/mm grating spectrometer. Using Gaussian fitting of both the X and XX lines, the FSS can be measured with sub-  $\mu\text{eV}$  resolution.

## B. Charge-noise and temperature dependence

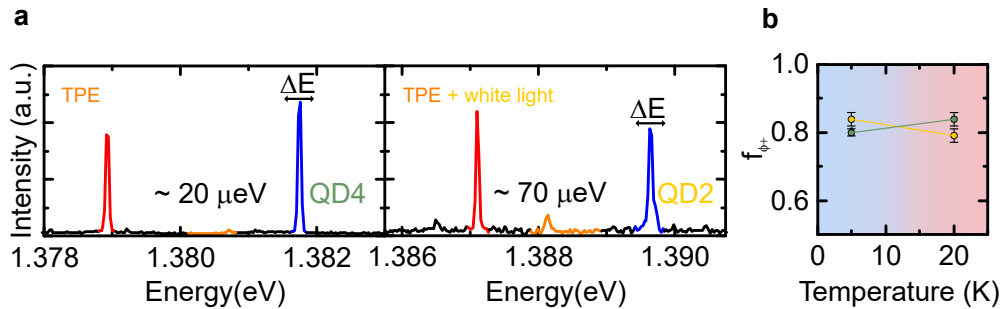

FIG. 2. (a) Photoluminescence spectra of two of the investigated QDs under resonant TPE, with the emitted XX (red) and X (blue) signals and the residual laser stray light (orange). QD4 (left panel) shows resolution-limited emission, while QD1 displays significant broadening most probably related to charge noise. The X linewidth (black) is reported in each panel. (b) Measured entanglement fidelity for temperatures of 5 K (standard for liquid He) and 20 K (liquid He plus counter-heating) for QD4 (green) and QD1 (yellow).

Fluctuating charges in the vicinity of the QD were determined as a source of line-

broadening in QDs, with a noise-spectrum up to the kHz-range [7, 8]. As long as these fluctuations couple equally to the two possible X angular-momentum-eigenstates, their energy levels shift in unison and thus no dephasing between the two X states is expected. To test this claim, we further investigate QD1 and QD4, which underlie vastly different charge-noise conditions, as evident from the spectra in Fig. 2(a): QD4 (left panel) emits signal with a linewidth corresponding to the spectrometer’s resolution limit of  $\lesssim 20 \mu\text{eV}$ , while QD1 (right panel) suffers from substantially higher charge-noise, resulting in a linewidth of about  $70 \mu\text{eV}$ . However, despite the large difference in charge-environment, both QDs’ measured  $f$  values lie close to the expected values from Eq. 7 in the main paper, so that we exclude significant degradation of entanglement due to charge-noise.

Finally, we investigate the role of temperature as a possible entanglement-degrading effect. Figure 2(b) shows the measured  $f$  of QD1 and QD4, each for two different temperatures of 5 K and 20 K. No significant change in  $f$  is observed, which is incompatible with a strong phonon-dependent effect, which we thus rule out as an important dephasing channel in the QDs measured in this work.

### C. XX inversion efficiency

For an unpolarized pair of photons from the same decay cascade the coincidence rate scales linearly with the pair-emission probability  $\eta_P$ , while the coincidence rate between different excitation cycles scales with  $\eta_P^2$ . Comparing the number of events from four different XX-X cross-polarization measurements at  $\tau = 0$  with the average of the events at different  $\tau$  (the side-peaks) therefore allows to deduce the XX inversion efficiency per pulse  $\eta_P$ , according to the following equation:

$$\frac{1}{\eta_P} = \sum_j \frac{A_j^0}{A_j^S}, \quad j \in \{\text{HH}, \text{HV}, \text{VH}, \text{VV}\}, \quad (18)$$

where  $A_0$  is the area of the middle peak of the correlation histogram and  $\langle A_S \rangle$  is the average side-peak area.

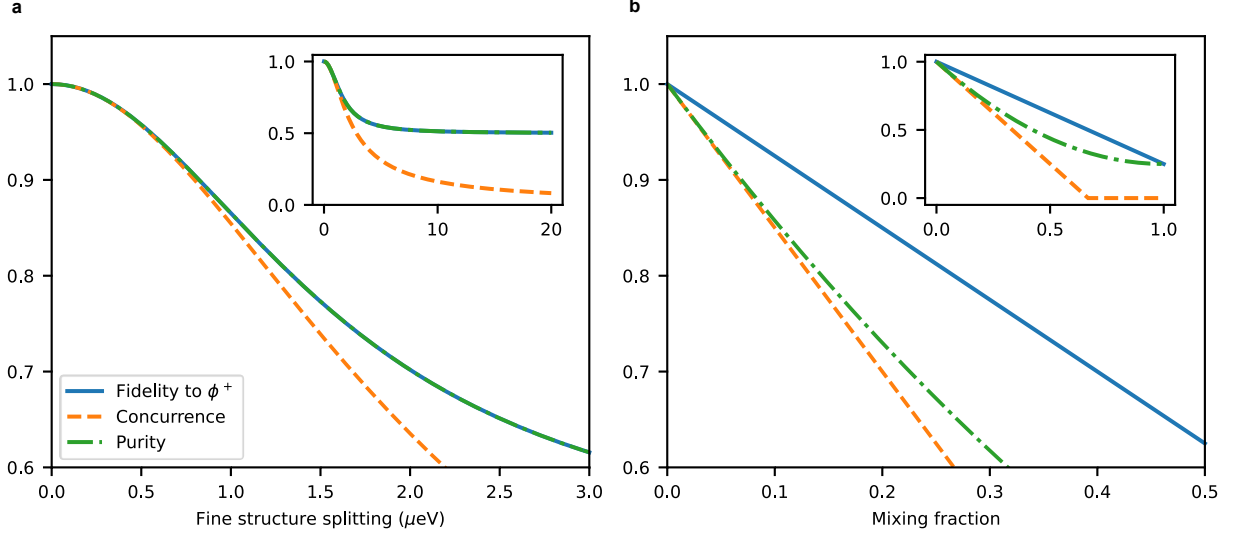

FIG. 3. (a) Effect of pure dephasing, simulated by an increasing fine structure splitting (FSS) in a QD with a lifetime of 433 ps, on the fidelity, concurrence, and purity of the calculated two-photon state. The inset shows the same data, but in a broader FSS range. (b) Effect of a mixing channel with varying mixing fraction from zero (maximum entangled state) to one (perfectly mixed state) on the fidelity, concurrence and purity on the calculated two-photon state. The inset shows the same data, but with higher range of the mixing fraction.

#### D. Dependence of entanglement on FSS in presence of pure dephasing and state mixing

Figure 3 shows a comparison of the effect pure dephasing and state mixing have on the quantities derived from the two-photon density matrix as a function of FSS (or any other energy difference between the bright X states). Pure dephasing channels [Fig. 3(a)], caused by adiabatic shifts of the X energy levels, lead to a similar initial drop for fidelity, purity and concurrence for FSS below 1  $\mu\text{eV}$  for an X lifetime of 433 ps. The purity and the fidelity behave equally and converge to 0.5 in the limit of high FSS, and the concurrence approaches zero. In the case of state mixing [Fig. 3(b)], which can stem from imperfect single photon emission or spin flip-flop processes (“spin scattering”), the purity and the concurrence deviate strongly from the fidelity already for small mixing fractions. A strong discrepancy between the fidelity and the concurrence, as reported in the main paper, can therefore be an indicator for a mixing channel at play. Further evidence for additional mixing

channels, not captured by the OS model, is found in previous studies of InGaAs QDs [9–11], where, in the limit of high  $S$ , the fidelity converges towards 0.45, and not to 0.5.

## V. QUANTUM DOT DETAILS

### A. Degree of linear polarization of the XX and X emission

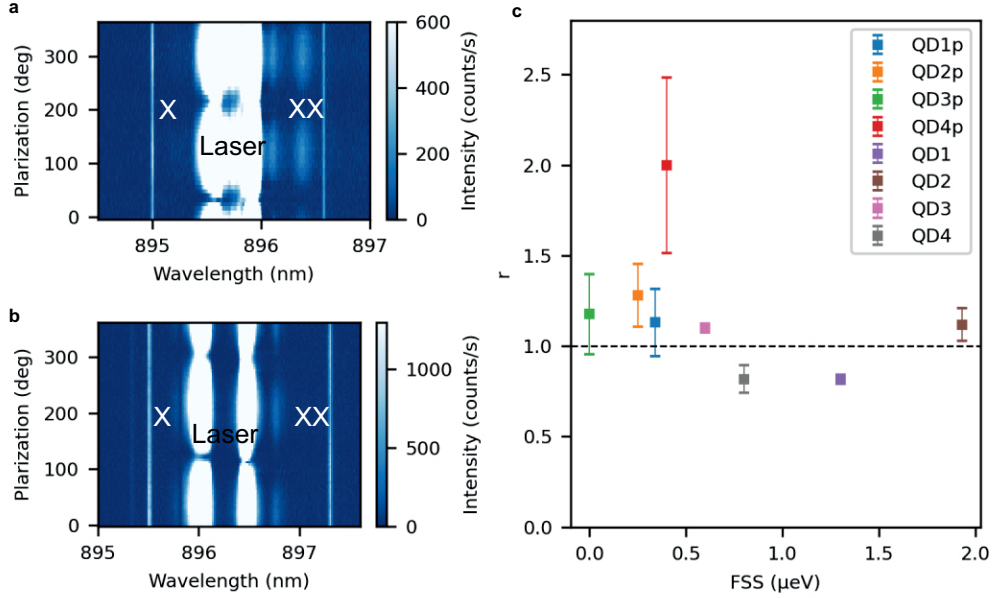

FIG. 4. (a) Polarization-resolved emission of QD1p excited via TPE under  $\pi$ -pulse condition. The degree of linear polarization (DOLP) of the X signal is 0.224(4), while for XX the DOLP is within the error (0.004). (b) Emission of QD3p. The X and XX exhibit a DOLP of 0.019(7) and 0.111(7), respectively. (c) Ratio of fitted intensities  $r = I_X/I_{XX}$  between the X and the XX. The squared symbols correspond to the average  $\langle r \rangle$  over all polarizations in the polarization-map, the bars correspond to the maximum and minimum measured  $r$  within the whole polarization map.

### B. Measured parameters used in the model

TABLE I. Summary of the measured multi-photon emission probabilities under TPE of XX and X photons for all QDs investigated in this work.

| As-grown QDs  |                               |                           |
|---------------|-------------------------------|---------------------------|
| QD 1          | $g_{XX}^{(2)}(0) = 0.009(3)$  | $g_X^{(2)}(0) = 0.008(2)$ |
| QD 2          | $g_{XX}^{(2)}(0) = 0.021(4)$  | $g_X^{(2)}(0) = 0.031(7)$ |
| QD 3          | $g_{XX}^{(2)}(0) = 0.018(4)$  | $g_X^{(2)}(0) = 0.008(2)$ |
| QD 4          | $g_{XX}^{(2)}(0) = 0.013(4)$  | $g_X^{(2)}(0) = 0.009(3)$ |
| Processed QDs |                               |                           |
| QD 1 $p$      | $g_{XX}^{(2)}(0) = 0.036(7)$  | $g_X^{(2)}(0) = 0.008(3)$ |
| QD 2 $p$      | $g_{XX}^{(2)}(0) = 0.029(9)$  | $g_X^{(2)}(0) = 0.029(7)$ |
| QD 3 $p$      | $g_{XX}^{(2)}(0) = 0.043(15)$ | $g_X^{(2)}(0) = 0.014(7)$ |
| QD 4 $p$      | $g_{XX}^{(2)}(0) = 0.014(3)$  | $g_X^{(2)}(0) = 0.015(4)$ |

TABLE II. Summary of the measured radiative lifetimes under TPE of XX and X photons for all QDs under investigation. The values are obtained after convolution with the instrument's response function and an exponential (XX) or double-exponential (X) for each decay curve.

| As-grown QDs  |                              |                            |
|---------------|------------------------------|----------------------------|
| QD 1          | $T_1^{XX} = 165(4)\text{ps}$ | $T_1^X = 464(13)\text{ps}$ |
| QD 2          | $T_1^{XX} = 150(4)\text{ps}$ | $T_1^X = 346(8)\text{ps}$  |
| QD 3          | $T_1^{XX} = 166(5)\text{ps}$ | $T_1^X = 327(10)\text{ps}$ |
| QD 4          | $T_1^{XX} = 168(4)\text{ps}$ | $T_1^X = 369(7)\text{ps}$  |
| Processed QDs |                              |                            |
| QD 1 $p$      | $T_1^{XX} = 208(7)\text{ps}$ | $T_1^X = 433(13)\text{ps}$ |
| QD 2 $p$      | $T_1^{XX} = 199(6)\text{ps}$ | $T_1^X = 461(13)\text{ps}$ |
| QD 3 $p$      | $T_1^{XX} = 219(7)\text{ps}$ | $T_1^X = 495(13)\text{ps}$ |
| QD 4 $p$      | $T_1^{XX} = 208(5)\text{ps}$ | $T_1^X = 505(11)\text{ps}$ |

TABLE III. Summary of the measured entanglement fidelity to the expected Bell state for different values of the FSS for all QDs investigated

| As-grown QDs |                               |                                |
|--------------|-------------------------------|--------------------------------|
|              | FSS ( $\pm 0.2\mu\text{eV}$ ) | $f_{\phi^+}^{\text{measured}}$ |
| QD 1         | $1.3\mu\text{eV}$             | 0.83(1)                        |
| QD 2         | $1.9\mu\text{eV}$             | 0.52(2)                        |
| QD 3         | $0.6\mu\text{eV}$             | 0.83(1)                        |
| QD 4         | $0.8\mu\text{eV}$             | 0.79(1)                        |

  

| Processed QDs |                               |                                |
|---------------|-------------------------------|--------------------------------|
|               | FSS ( $\pm 0.2\mu\text{eV}$ ) | $f_{\phi^+}^{\text{measured}}$ |
| QD 1 $p$      | $0.3\mu\text{eV}$             | 0.89(1)                        |
| QD 2 $p$      | $0.3\mu\text{eV}$             | 0.90(1)                        |
| QD 3 $p$      | $0.2\mu\text{eV}$             | 0.86(1)                        |
| QD 4 $p$      | $0.2\mu\text{eV}$             | 0.64(4)                        |

## REFERENCES

---

- [1] M. Bayer, G. Ortner, O. Stern, A. Kuther, A. A. Gorbunov, A. Forchel, P. Hawrylak, S. Fafard, K. Hinzer, T. L. Reinecke, S. N. Walck, J. P. Reithmaier, F. Klopff, and F. Schäfer, Fine structure of neutral and charged excitons in self-assembled In(Ga)As/(Al)GaAs quantum dots, *Phys. Rev. B* **65**, 195315 (2002).
- [2] E. Weland, J. Hildmann, and G. Burkard, Influence of hyperfine interaction on the entanglement of photons generated by biexciton recombination (2014), arXiv:1409.6521.
- [3] B. Eble, C. Testelin, P. Desfonds, F. Bernardot, A. Balocchi, T. Amand, A. Miard, A. Lemaître, X. Marie, and M. Chamarro, Hole-nuclear spin interaction in quantum dots, *Phys. Rev. Lett.* **102**, 146601 (2009).
- [4] J. Neuwirth, F. B. Basset, M. B. Rota, J.-G. Hartel, M. Sartison, S. F. C. da Silva, K. D. Jöns, A. Rastelli, and R. Trotta, A multipair-free source of entangled photons in the solid state, *Phys. Rev. B - Condens. Matter Mater. Phys.* **106**, L241402 (2022).
- [5] L. Wang, A. Rastelli, and O. G. Schmidt, Structural and optical properties of In(Ga)As/GaAs quantum dots treated by partial capping and annealing, *Journal of Applied Physics* **100**, 064313 (2006).
- [6] Y. M. He, Y. He, Y. J. Wei, D. Wu, M. Atatüre, C. Schneider, S. Höfling, M. Kamp, C. Y. Lu, and J. W. Pan, On-demand semiconductor single-photon source with near-unity indistinguishability, *Nat. Nanotechnol.* **8**, 213 (2013).
- [7] A. V. Kuhlmann, J. Houel, A. Ludwig, L. Greuter, D. Reuter, A. D. Wieck, M. Poggio, and R. J. Warburton, Charge noise and spin noise in a semiconductor quantum device, *Nat. Phys.* **9**, 570 (2013).
- [8] C. Schimpf, M. Reindl, P. Klenovský, T. Fromherz, S. F. Covre Da Silva, J. Hofer, C. Schneider, S. Höfling, R. Trotta, and A. Rastelli, Resolving the temporal evolution of line broadening in single quantum emitters, *Opt. Express* **27**, 35290 (2019).
- [9] A. J. Hudson, R. M. Stevenson, A. J. Bennett, R. J. Young, C. A. Nicoll, P. Atkinson, K. Cooper, D. A. Ritchie, and A. J. Shields, Coherence of an entangled exciton-photon state, *Phys. Rev. Lett.* **99**, 266802 (2007).

- [10] R. Trotta, J. S. Wildmann, E. Zallo, O. G. Schmidt, and A. Rastelli, Highly entangled photons from hybrid piezoelectric-semiconductor quantum dot devices, *Nano Lett.* **14**, 3439 (2014).
- [11] J. Zhang, J. S. Wildmann, F. Ding, R. Trotta, Y. Huo, E. Zallo, D. Huber, A. Rastelli, and O. G. Schmidt, High yield and ultrafast sources of electrically triggered entangled-photon pairs based on strain-tunable quantum dots, *Nature communications* **6**, 1 (2015).
